# Supplementary material for: A Stochastic Geometry Framework for Performance Analysis of RIS-assisted OFDM Cellular Networks
Source: arXiv:2310.06754 source file (2026-10-11)
Supplement: Supplementary file 1 [file 5_numerical_supplement.tex]

\subsubsection{RISs need strategic placement near either BS or UE}
\todo[inline]{Reviewer 3 raised concerns about the justification for our claim that RISs should be placed near BS or UE, citing limitations in existing literature that relies on 1D scenarios rather than our 2D modeling. 
We can address this gap by providing a simulation using our framework that justifies the statement on the RIS placement strategy.}

\begin{figure}[htp]
    \centering
    \includegraphics[width=0.6\linewidth]{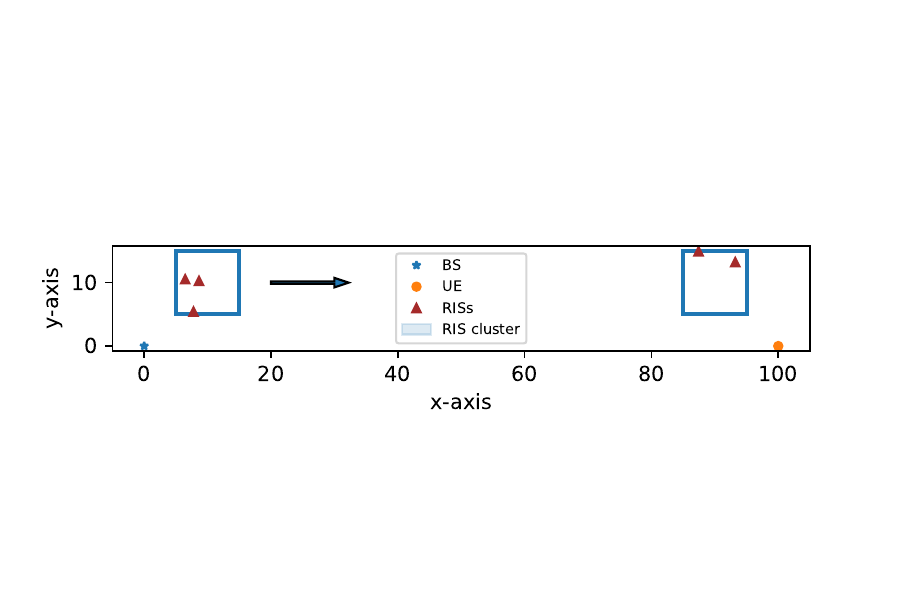}
    \caption{Strategies for randomly deploying RISs in a square area}
    \label{fig:proximity}
\end{figure}
\begin{figure}
    \centering
    \includegraphics[width=0.5\linewidth]{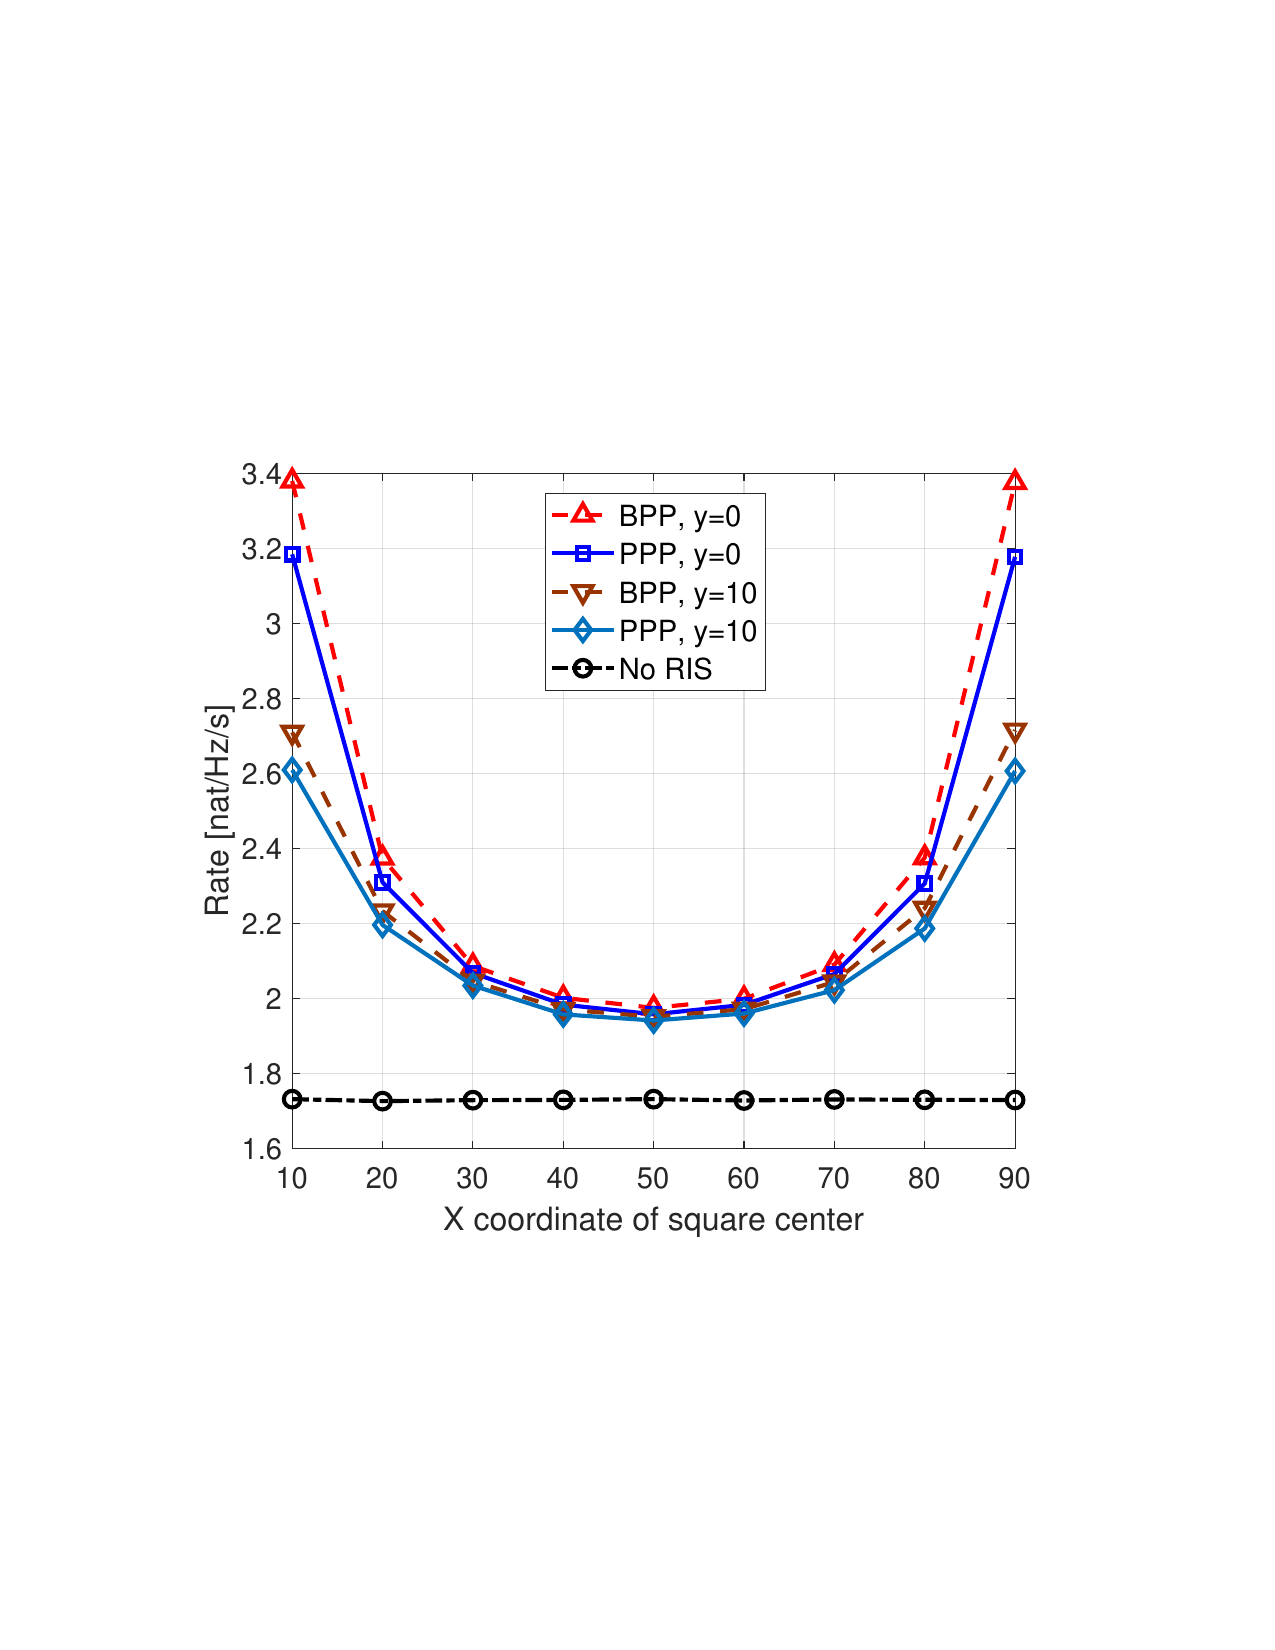}
    \caption{Impact of RIS deployment in square area on system performance}
    \label{fig:nearFar}
\end{figure}

In Fig.~\ref{fig:proximity}, we consider a scenario where multiple RISs are deployed in a square area. When we investigate the impact of spatial deployment by varying the center location of this square. 
Here, the x-direction refers to the line from the UE (located at $(0, 0)$ ) to the BS (located at $(100, 0)$ ), and the y-direction is perpendicular to this line. 
Outside the cell guaranteeing this association, we assume that interfering BSs follow the PPP model considered in this paper.
To model randomly located RISs, we model them as either a BPP with a constant number of RISs $N_{\rm RIS}=2$ or a PPP with a average number of RISs equal to $\lambda_{\rm RIS} = 2/{\rm (Area~of~square)}.$
We assume that each RIS has $M=3000$ elements and that there are $5$ UEs are in this cell. 
In other words, each RIS serves each UE using $M_o=600$ elements to form a narrow reflecting beam.
It is shown in Fig.~\ref{fig:nearFar} that the ergodic rate improvement due to RISs is most significant when the center of the square region is close to either the BS or the UE.
Two phenomena can characterize this trend: the rate enhancement becomes more significant when the x-coordinate approaches either 10 (namely, the RISs are close to the UE) or 90 (close to the BS). 
On the other hand, when we analyze the y-coordinate, the set of curves of a y-coordinate of 0 is above that of a y-coordinate of 10, further validating the proximity deployment guideline.
The same trend applies to the models of the BPP and the PPP.
We can conclude that for the RIS deployment to effectively reflect the received signal, RISs should be placed in the proximity of either BSs or UEs.
In addition, by comparing the curves representing BPP modeling with that of the PPP modeling, one sees that deploying a fixed number of RISs in the pre-defined area can provide a higher gain in terms of ergodic rate than the improvement due to deploying a random number of RISs. 
However, several real-world uncertainties can affect the planned deployment of RISs in an area. 
For example, the lack of mounting structures makes it difficult to guarantee an exact number of RISs. 
Therefore, modeling RISs as PPPs improves the generality and flexibility of investigating the influence of RISs.
